# Supplementary material for: Privacy Amplification via Shuffled Check-Ins
Source: arXiv:2206.03151 source file (2023-07-04)
Supplement: Supplementary file 1 [file app_additional.tex]

\section{Code for Reproducibility}
\label{app:code}
See \url{https://anonymous.4open.science/r/checkin-B2B1/} for the code of our implementation.

\section{Additional Privacy Analyses}
\label{app:add}
\subsection{Distributed check-in under removal DP}
\label{subsec:rm_dci}
As before, we assume that the server aggregates the received messages by outputting the average, $\frac{1}{B}\sum_{i=1}^B x_i + \mathcal{N}(0,\sigma^2/B)$.
The mechanism is closely related to Poisson subsampling \citep{zhu2019poission}.

\begin{theorem}
[Distributed check-in Gaussian RDP (removal DP)]
Consider the mechanism in Equation \ref{eq:cci} where agg is a mean operation on collected values.
Here it is assumed that the adversary does not know the number of user checking in in each round.
\begin{align}
\eps(\lambda) &\leq \frac{1}{1-\lambda}\log \{(1-\gamma)^{\lambda-1}(\lambda\gamma-\gamma+1) \nonumber \\
&+ \sum_{k=1}^{n-1}\binom{\lambda}{2}\binom{n-1}{k}\gamma^{k+2} (1-\gamma)^{n+\lambda-3-k} e^{\eps_k^{\rm CCI}(2)} \label{eq:poiss1} \\
&+ \binom{\lambda}{2}(1-\gamma)^{n+\lambda-3}\gamma^2 e^{1/\sigma^2} + 3 \sum_{l=3}^\lambda\binom{\lambda}{l} \gamma^{\lambda-l} (1-\gamma)^{n+l-1}e^{l(l-1)/2\sigma^2} \nonumber \\
&+ 3\sum_{k=1}^{n-1}\sum_{l=3}^\lambda \binom{n-1}{k} \binom{\lambda}{l}\gamma^{k+\lambda-l} (1-\gamma)^{n+l-1-k}e^{(l-1)\eps_k^{\rm CCI}(l)}\} \label{eq:poiss2}
\end{align}
where $\exp((l-1)(\eps_k^{\rm CCI}(l)) = \sqrt{\frac{(k+1)^{l}}{(k+l)k^{l-1}}}\exp{(-\frac{l+1}{\sigma^2(k+1)})}$ for $k\geq 1 $.
% and $\eps_0^{\rm CCI}(l) = l/2\sigma^2$.
Line \ref{eq:poiss1} can be further approximated as
\begin{align}
   \binom{\lambda}{2}\gamma^2 (1-\gamma)^{\lambda-2} \left(e^{\eps_{1}^{\rm CCI}(2)-\Delta^2(n-1)\gamma/2} + e^{\eps_{(1-\Delta)(n-1)\gamma+1}^{\rm CCI}(2)}\right)
\end{align}
and Line \ref{eq:poiss2} can be further approximated as
\begin{align}
% \eps(\lambda) &\leq \frac{1}{1-\lambda}\log \{(1-\gamma)^{\lambda-1}(\lambda\gamma-\gamma+1) \nonumber \\
% &+ \binom{\lambda}{2}\gamma^2 (1-\gamma)^{\lambda-2} e^{\eps^{\rm CCI}(2)} + 3 \sum_{l=2}^\lambda (1-\gamma)^{n-1}(1-\lambda)^{l}\lambda^{\lambda-l}e^{l(l-1)/2\sigma^2} \nonumber \\
3\sum_{l=2}^\lambda  \binom{\lambda}{l}(1-\gamma)^{l}\gamma^{\lambda-l}(e^{(l-1)\eps_{1}^{\rm CCI}(l)-\Delta^2(n-1)\gamma/2}+e^{(l-1)\eps_{(1-\Delta)(n-1)\gamma+1}^{\rm CCI}(l)})
\end{align}
where $\Delta \in [0,1]$.
\end{theorem}
\begin{proof}
The neighboring databases are $D$, $D' = D \cup \{x\}$, and the mechanisms acting on them are $\mathcal{M},\mathcal{M'}$ respectively.
Let $J$ be the index set indicating whether a user participates in training, $J=  (\sigma_1,\sigma_2,\cdots,\sigma_n) \in \{0,1\}^n$.
Let $\mathbb{P}(J)$ be the probability distribution of $J$.

We denote $q(J)$ by the underlying randomization mechanism, which is a Gaussian mechanism with variance $\sigma^2/k$, $k$ being the number of non-zero elements in $J$.
Following \cite{zhu2019poission}, we define $q' = \sum_J q'(J), q'(J) = q(\sigma_1, \cdots, \sigma_{n-1}, 1)$, and similarly $p(J)=p'(J) = q(\sigma_1, \cdots, \sigma_{n-1}, 0)$.
We have $q = (1-\gamma)p + \gamma q'$ or $p = q+\gamma p'-\gamma q'$.

we want to calculate the RDP of neighboring databases $\mathcal{M}\sim p$, $\mathcal{M'}\sim q$:
\begin{align*}
&\mathbb{E}_{\mathcal{M'}}\left[(\mathcal{M}/\mathcal{M'})^\lambda\right] = \mathbb{E}_q \left[\left(\frac{q+\gamma p'-\gamma q'}{q}\right)^{\lambda}\right] \\
& \leq \mathbb{E}_{\sigma_1,\dotsc,\sigma_{n-1}} \{\gamma \mathbb{E}_{q'(J)}\left(\frac{(1-\gamma)q'(J)+\gamma p'(J)}{q'(J)}\right)^{\lambda}  + (1-\gamma) \mathbb{E}_{p'(J)}\left(\frac{(1+\gamma)p'(J)-\gamma q'(J)}{p'(J)}\right)^{\lambda} \} \\
& = \sum_{k=0}^{n-1}\sum_{l=0}^{\lambda} \binom{\lambda}{l} \binom{n-1}{k}\gamma^k (\gamma)^{n-1-k}  (1-\gamma)^{\lambda-l}\gamma^l \left\{\gamma\mathbb{E}_{q'(k)} \left(\frac{{p'(k)}}{{q'(k)}}\right)^{l} + (1-\gamma)\mathbb{E}_{p'(k)}\left(2-\frac{{q'(k)}}{{p'(k)}}\right)^{l}\right\}
\end{align*}
Here, $q'(k)\sim \mathcal{N}(1/(k+1),\sigma^2/(k+1))$, $p'(k)\sim \mathcal{N}(0,\sigma^2/k)$ when $k\geq 1$.
By direct computation $\mathbb{E}_{q'(k)}(p'(k)/q'(k))^{\lambda} = \sqrt{\frac{(k+1)^{\lambda}}{(k+\lambda)k^{\lambda-1}}}\exp{(-\frac{\lambda+1}{\sigma^2(k+1)})}$. 
When $k=0$, $q'(k)\sim \mathcal{N}(1,\sigma^2)$, $p'(k)\sim \mathcal{N}(0,\sigma^2)$ and $\mathbb{E}_{q'(k)}(p'(k)/q'(k))^{\lambda} = \exp{[(\lambda^2-\lambda)/(2\sigma^2)]}$.

Moreover, from Lemma \ref{lm:chernoff}, we can make the approximation of lines \ref{eq:poiss1} and \ref{eq:poiss2}.
% From the Chernoff bound:  $\mathbb{P}[X \leq (1-\Delta)\mu] \leq e^{-\Delta^2\mu/2}$ for all $\Delta \in [0,1]$ and the union of probability, we can make the approximation of lines \ref{eq:poiss1} and \ref{eq:poiss2}.

We can then use the same argument in \cite{zhu2019poission} to obtain the desired result.

% We can write $\tilde{q}(k) = \sum_{J}\mathbb{P}(J)q(J)\delta(\sum_i\sigma_i=k)=\binom{n}{k}\gamma^k(1-\gamma)^{n-k}\mathcal{N}(1/k,\sigma^2/k)$.
\end{proof}
\begin{remark}
One can obtain a tighter bound if $\mathbb{E}_{q'(k)}(p'(k)/q'(k)-1)^{\lambda}\geq 0$ for odd $\lambda$ \citep{zhu2019poission}.
Unfortunately this does not apply to our scenario as $\mathbb{E}_{q'(k)}(p'(k)/q'(k)-1) <0$ by direct computation.
\end{remark}

\subsection{Shuffled check-in with a generic $(\eps_0,\delta_0)$-LDP randomizer}
Here, we give another approach of privacy accounting of shuffled check-in with a generic $(\eps_0,\delta_0)$-LDP randomizer, following arguments given at the end of Section \ref{subsec:rdp_sci}.

\noindent\textbf{Shuffling conversion.}
\begin{enumerate}
    \item Convert shuffle DP to shuffle RDP.
    \item Use shuffle RDP to evaluate subsampled shuffle RDP
    \item Substitute it into Equation \ref{eq:main} to evaluate the composition of RDP.
\end{enumerate}
To calculate the shuffle DP with $(\eps_0,\delta_0)$-LDP randomizer, we use Theorem 3.8 given by \cite{feldman2022hiding}. 
% \footnote{\label{fn:shuff}.
% The result of privacy amplification by shuffling by \cite{feldman2022hiding} is valid only when $\eps_0 \leq \log\left(n/16\log(2/\delta)\right)$. For parameters violating this condition, we assume that no amplification occurs, i.e., $\eps=\eps_0$. 
% This is well corroborated by the numerical experiments performed in \cite{feldman2022hiding}.}
The subsampled RDP can be calculated using Theorem 9 of \cite{wang2019subsampled}.

Note that Step 2 is a calculation of $O(\lambda)$ in terms of time complexity \citep{wang2019subsampled}.
Step 3 involves evaluating the summation with respect to $n$ as in Equation \ref{eq:main}, which is of $O(n)$.
One also needs to convert the RDP notion back to approximate DP using Lemma \ref{lm:rdpdp}, which is an $O(\lambda)$ operation.
% Overall, the shuffling conversion approach is of time complexity $O(n\lambda^2)$. \footnote{Here, we do not include the time complexity of optimizing Equation \ref{eq:dprdp} for convenience as it is irrelevant to the subsequent discussions.
% We note however that Equation \ref{eq:dprdp} is convex optimization problem which can be solved efficiently.}

% Table \ref{tab:comp} summarizes the 
Table \ref{tab:comp} summarizes the two approaches introduced in this paper.
Although the subsampling shuffling conversion approach has lower time complexity, we expect the RDP bound to be looser than the shuffling conversion approach as the conversion to RDP occurs one step later.

\begin{table}
\begin{center}
\caption{Our approaches to bounding shuffled check-in mechanism with a generic $(\eps_0,\delta_0)$-LDP randomizer.
Here, A, B, C, D refer to techniques used in \cite{feldman2022hiding}, \cite{wang2019subsampled}, \cite{balle2018privacy},  \cite{balle2018privacy}, respectively.
See text for details.
    The conversion from DP to RDP (using Lemma \ref{lm:dprdp}) can be performed in two different steps leading to different time complexities as shown in the Table.
    Dependence of the time complexity on other factors is suppressed.}
    \label{tab:comp}

    \begin{tabular}{ccccc}
        \toprule
        %\multirow{2}{*}{Dataset} &  \multicolumn{3}{c|}{social}& comm & web \\
        
         &Shuffling&  Subsampling& Convert to RDP from & Time complexity \\
                \midrule
      Shuff. conv.& Use A (DP) &Use B (RDP)& A& $O(n\lambda^2)$ \\
      Subs. shuff. conv.& Use A (DP)& Use C (DP)& A+D& $O(n \lambda)$ \\
    %   Processing complexity& -& $n^2$& $O(\log(n))$ \\
        \bottomrule
    \end{tabular}
    
\end{center}
% \vspace{-0.2cm}
\end{table}
